# Supplementary material for: Generating Prototypes for Contradiction Detection Using Large Language Models and Linguistic Rules
Source: arXiv:2310.14732 source file (2023-10-23)
Supplement: Supplementary file 1 [file appendix.tex]

\label{appendix}
